# Supplementary material for: Bifurcation analysis of multiple limit cycles created in boundary equilibrium bifurcations in hybrid systems
Source: arXiv:2412.06911 source file (2024-12-09)
Supplement: Supplementary file 1 [file Appendix-I.tex]

%! Author = ib20968
%! Date = 2/11/2024
% ----------------------------------------------------------------------------------------------

\section{Numerical evaluation of the return map}\label{sec:numerical-evaluation-of-the-return-map}
\begin{algorithm}[h]
        \LinesNumbered
        \KwData{Matrix $\mathbf{A}$, reset map matrix $\mathbf{P}$, searching region $[0,~t_{\rm end}]$, stepsize
            $\Delta
            t$, tolerance ${\rm [tol]}$.}
        \KwResult{ $\mathcal{N}$, the number of LCOs found; $\{ \mathbf{\hat{y}}_{\rm i}, T_{\rm i}, \mathcal{M}_{\rm
        i},
        \mathcal{S}_{\rm i}\}, \; (i =1,\cdots, \mathcal{N})$ for each LCO, with initial condition
            $\mathbf{\hat{y}}_{\rm
            i}$, corresponding period $T_{\rm i}$,  the corresponding biggest Floquet multiplier $\mathcal{M}_{\rm
            i}$, and
            the value of $\hat{\mu}$ as $\mathcal{S}_{\rm i}$. }
        \tcc{Initialization }
        $ \tau \leftarrow 0, i \gets 0$ \;

        ${\rm \mathcal{N}} \gets 0, ~ \hat{\mathbf{y}} \gets [~], ~ \mathbf{T} \gets [~], ~ \mathcal{M} \gets [~],
        ~\mathcal{S} \gets [~],~ P \gets [~], ~ t \gets [~]$\;

        %$\Delta B^{\ast}\gets -\infty$\;
        \tcc{Begin search in given range}
        \SetKwFunction{FRMP}{ReturnMap}
        \SetKwFunction{FJac}{Jacobian}
        \SetKwFunction{FSt}{store}
        \SetKwFunction{FLReig}{LReig}

        \SetKwProg{Fn}{Function}{:}{}
        \Fn{\FRMP{prob, $\mu$, $\eta$, IC}}{
            \tcc{Numerically marching the system \cref{eq:composedReturnMap} in time until the returning condition
            \cref{eq:returning_condition} and the state $u_*^r$ on the poincar\'e section is captured by the built-in
            event
            detection functionality }

            \KwRet $u_*^r$ \;
        }\;
        \Fn{\FJac{prob, $\hat{u}$ }}{
        %\tcc{Compute the Jacobian of the return map at fixed point for given $\mu_0, \eta_0$}
            ind =  prob.ind defines the index of the  \;

            \For(\tcc*[h]{traversal perturbation to each component of $\hat{u}$ }){i = length$(\hat{u})$}
            {
                tol     = 1, \; $Jac\_tmp = 0$, \; h = 1, \;S  = zeros(size($\hat{y}$)),\; S(ind(i)) = 1;

            \While{$h > 1e-9$}{

                $\displaystyle Jac_{new} \gets \frac{ \FRMP(prob, \mu_0, \eta_0, \hat{y}+Sh) - \FRMP(prob, \mu_0,
                \eta_0,
                \hat{y}-Sh) }{2h} $ \;

                $\displaystyle tol \gets \frac{||Jac_{new} - Jac_{tmp}||_2}{||Jac_{tmp}||_2}$

                \If{$tol < 1e-6$}{
                    break;
                }

                $Jac_{tmp} \gets Jac_{new} $,\; $h \gets h/2$\;
            }
            }
            $Jac(:,i) \gets Jac\_new$  \;

            \KwRet $Jac$\;
        }

        \caption{Return map expansion numerical implements:part I}
        \label{alg:RMap_expansion_p1}
    \end{algorithm}
%> the second part of the algorithm
    \begin{algorithm}
        \LinesNumbered
        \setcounter{AlgoLine}{16}
        %% This is to restore vline mode if you did not take the package as \usepackage[linesnumbered,ruled,
        %% vlined]{algorithm2e}
        \SetAlgoVlined
        \tcc{Compute the expansion around the fixed point in the eigen direction $v$ of Jac
        corresponding to -1/1 Floquet multiplier }

        $Jac \gets \FJac(prob, \hat{u} );(w,v) \gets \FLReig(Jac)$ \tcc*[h]{obtain the left/right eigen vectors}\;

        \tcc{approximate the derivatives regarding the $z$ coordinate}\;
        $\lambda_{tmp}  \gets 0;
        c_{tmp}       \gets 0;
        d_{tmp}       \gets 0;
        a_0^{tmp}       \gets 0;
        b_0^{tmp}       \gets 0;
        a_1^{tmp}       \gets 0;
        b_1^{tmp}       \gets 0;
        $ \;

        $tol_{\lambda}  \gets 1;
        tol_c       \gets 1;
        tol_d       \gets 1;
        h \gets 1 ;$ \;

        \While{$ h > 10^{-12}$ }
        {
            $F(x,\delta_{\mu},\delta_{\eta})   \coloneq  \FRMP(prob, \mu_0 +\delta_{\mu}, \eta_0 +\delta_{\eta},
            \hat{u}+xv);
            $ \;

            $\displaystyle a_0^{new} \gets \frac{w^{\top} (F(0,h,0) - F(0,-h,0))}{2h}$
            \tcc*[h]{approximate $\frac{\partial \hat{p}}{\partial \mu}$ term}\;

            $\displaystyle b_0^{new} \gets \frac{w^{\top} (F(0,0,h) - F(0,0,-h))}{2h}$
            \tcc*[h]{approximate $\frac{\partial \hat{p}}{\partial \eta}$ term}\;

            $\displaystyle a_1^{new} \gets \frac{w^{\top} (F(h,h,0) + F(-h,-h,0) -F(h,-h,0) - F(-h,h,0))}{4h^2}$
            \tcc*[h]{ $\cdots \frac{\partial \hat{p}^2}{\partial \mu\partial z}$ term}\;

            $\displaystyle b_1^{new} \gets \frac{w^{\top} (F(h,0,h) + F(-h,0,-h) -F(h,0,-h) - F(-h,0,h))}{4h^2}$
            \tcc*[h]{ $\cdots \frac{\partial \hat{p}^2}{\partial \eta\partial z}$ term}\;

            $\displaystyle \lambda_{new} \gets \frac{w^{\top} (F(h,0,0) - F(-h,0,0))}{2h}$ \tcc*[h]{approximate the
        first
        derivative $\frac{\partial \hat{p}}{\partial z}$}\;

            $\displaystyle c_{new} \gets  \frac{w^{\top}(F(h,0,0) + F(-h,0,0) - 2\hat{u})}{h^2}$ \tcc*[h]{$\cdots$second
            $\cdots$ $ \frac{\partial \hat{p}^2}{\partial^2 z}$} \;

            $\displaystyle d_{new} \gets \frac{w^{\top} (F(2h,0,0) -F(-2h,0,0)-2F(h,0,0) + 2F(-h,0,0))}{2h^3}$
            \tcc*[h]{$\cdots$third$\cdots$}\;

            $\displaystyle tol_1 \gets \frac{|\lambda_{new} - \lambda_{tmp}|}{|\lambda_{new}|}; \;
            tol_2 \gets \frac{|c_{new} - c_{tmp}|}{|c_{new}|}; \;
            tol_3 \gets \frac{|d_{new} - d_{tmp}|}{|d_{new}|}; \;
            tol_4 \gets \frac{|a_0^{new} - a_0^{tmp}|}{|a_0^{new}|}; $ \;

            $
            tol_5 \gets \frac{|b_0^{new} - b_0^{tmp}|}{|b_0^{new}|}; \;
            tol_6 \gets \frac{|a_1^{new} - a_1^{tmp}|}{|a_1^{new}|}; \;
            tol_7 \gets \frac{|b_1^{new} - b_1^{tmp}|}{|b_1^{new}|};
            $ \;

            $\lambda_{tmp} \gets \lambda_{new};\; c_{tmp} \gets c_{new};\; d_{tmp} \gets d_{new};\; h \gets h/2
            \tcc*[h]{update the variables}$\;

        \If{$tol_1 < tol_{\lambda}$}
        {
            $\lambda = \lambda_{tmp};\; tol_{\lambda} = tol_1$\;
        }

        \If{$tol_3 < tol_d$}
        {
            $d = d_{tmp};\; tol_d = tol_3$\;
        }

            $\vdots $ \tcc*[h]{repeat the same substitution process for the other approximators}\;

        \If(\tcc*{exit the loop with global accuracy met}){all of the tolerances become less than $10^{-6}$}
        {
            break;\;
        }

        }
        \tcc{Return the coefficients approximation for $z, z^2, z^3 $ terms}\;
        $ \lambda \gets \lambda;\; c \gets c/2;\; d \gets d/6;$\;

        \tcc{Return the coefficients approximation for $\mu, \eta, \mu z, \eta z $ terms}\;
        $ a_0 \gets a_0;\; b_0 \gets b_0;\; a_1 \gets a_1; \; b_1 \gets b_1;$\;
        \caption{Return map expansion numerical implements:part II}
        \label{alg:RMap_expansion_p2}
    \end{algorithm}

    \subsubsection{Comparison between the continuation curve and the analytical prediction}

%-----------------------------------------------------------------------------
    \begin{lemma}
        \label{lem:SN_PD_gradient}
        The condition \eqref{eq:PO_det_condition} defines a function $p(\mu,\eta,T) =0$ regarding the system parameter
        $\mu,
        \eta$    for the existence of period one impacting orbit.
        For our interest, we assume meanwhile a function $q(\mu,\eta,T) =0$ can be defined smoothly to determine the
        \emph{period-doubling/saddle} node bifurcations, where $q$ tracks the Floquet multiplier $-1$ or $1$ of the
        orbit's poincar\'e map respectively.
        Thus the two zero functions
        \begin{align}
            \label{eq:SN_PD_CO}
            \begin{split}
                p(\mu, \eta, T) &=  0,
                \\
                q(\mu, \eta, T) & = 0
            \end{split}
        \end{align}
        determines a codimension one curve $T = \tau(\mu,\eta)$.
        Being parameterized by the arc-length $s$, the curve can be writen in the form
        $$
        \mathbf{\Gamma} = \mu(s) \mathbf{j}+  \eta(s)\mathbf{k}+ T(s) \mathbf{i}
        $$
        whose tangent
        $\displaystyle \frac{\rm d \mathbf{\Gamma}}{ \rm d s}$
        is given by the tangent vector induced as the kernel of the Jacobian of
        \eqref{eq:SN_PD_CO} as $\mathbf{t} = [t_1, \;t_2, \; t_3]^{\top}$
        Then we can conclude that in the $(\mu,\eta)$ plane, the tangent of the codimension-2 curve $\eta(\mu)$ is
        given by $\displaystyle \frac{\rm d \eta}{\rm d \mu} = t_2/t_1$.
    \end{lemma}
%===============================================================================
